# Supplementary material for: Protected gap closing in Josephson junctions constructed on Bi$_2$Te$_3$ surface
Source: arXiv:1603.04540 source file (2018-09-11)
Supplement: Supplementary file 1 [file Supplementary_materials_single_JJ_160314.pdf]

**Supplementary Materials for**  
**“Observation of gap-closing on single Josephson junctions constructed**  
**on Bi<sub>2</sub>Te<sub>3</sub> surface”**

Yuan Pang<sup>1,\*</sup>, Junhua Wang<sup>1,\*</sup>, Zhaozheng Lyu<sup>1,\*</sup>, Guang Yang<sup>1</sup>, Jie Fan<sup>1</sup>, Guangtong Liu<sup>1</sup>,  
Zhongqing Ji<sup>1</sup>, Xiunian Jing<sup>1,2</sup>, Changli Yang<sup>1,2</sup> and Li Lu<sup>1,2†</sup>

*1 Beijing National Laboratory for Condensed Matter Physics, Institute of Physics,  
Chinese Academy of Sciences, Beijing 100190, People's Republic of China*

*2 Collaborative Innovation Center of Quantum Matter, Beijing 100871, People's Republic of China*

\* These authors contributed equally to this work.

† Corresponding authors: lilu@iphy.ac.cn

**Contents:**

1. Contact resistance obtained on another device with three Pd electrodes
2. Control experiment on Pb-Au-Pb Josephson devices
3. The mechanism of  $\pi$  phase shift in a single Josephson junction
4. The minigap in S-N-S Josephson junctions with different transparency to quasiparticle process
5. Estimation of effective junction area after considering flux compression

# 1. Contact resistance obtained on another device with three Pd electrodes

We have fabricated several devices with three contact positions in the junction area. Figure S1a shows the SEM image of one such device (named by device #S1). Figure S1b shows the differential resistance of contact position B and C. The blue curve (position B) shows a skewed oscillation against magnetic field, and the green curve (position C) shows an on/off-like oscillation. And all the curves are accompanied with abrupt jumps whenever flux passes the Fraunhofer nodes, in agreement with the data shown in the main manuscript.

Shown in Fig. S1c and d are the color plots of contact resistance measured at positions C and B, respectively, as functions of magnetic field and bias current. And shown in Fig. S1e and f are the line cuts of Fig. S1c and d respectively, as a function of bias current injected from the contact position. The results are similar to the ones presented in the main manuscript.

From Fig. S1e and f we can see that the red/pink curve shows clearly an enhanced resistance peak (a superconducting mini-gap structure), whereas the black/orange curve is gapless.

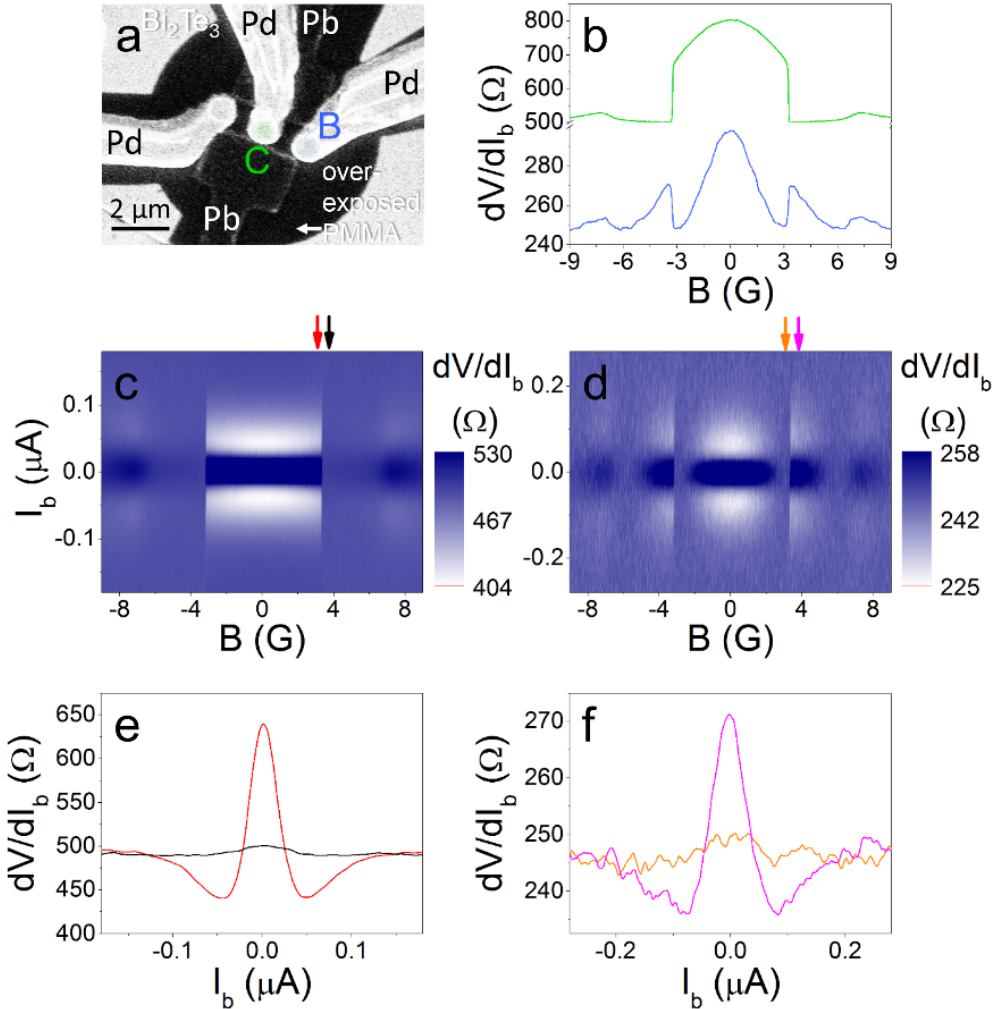

**FIG. S1** | (a) SEM image of device #S1. (b) Differential resistance of position C (green curve) and B (blue curve), respectively, as a function of magnetic field. (c), (d) Color plots of contact resistance measured at positions C and B, respectively, as functions of magnetic field and bias current. (e) The differential resistance curves of position C as a function of bias current before/after jumping. The colored curves are line cuts at the fields marked by the arrows of the same color in Fig. S1c. (f) The differential resistance curves of position B as a function of bias current before/after jumping. The colored curves are line cuts at the fields marked by the arrows of the same color in Fig. S1d. All the measurements were performed at  $\sim 20$  mK.

## 2. Control experiment on Pb-Au-Pb Josephson devices

We have fabricated several Pb-Au-Pb proximity-effect Josephson junctions, each with two point contact-like Pd electrodes to the two ends of the junction area on Au film, and performed transport measurements down to  $\sim 20$  mK or 200 mK. The results are similar. In the following we present the results obtained on one of such devices measured at 200 mK. The SEM picture of the device is shown in Fig. S2a. The supercurrent of this device demonstrates a standard Fraunhofer pattern for small Josephson junctions, as shown in Fig. S2b, with a critical supercurrent of up to  $\sim 100$   $\mu$ A. Figures S2c and S2d show the contact resistance  $dV/dI_b$  of the Pd electrodes at the upper and lower ends of the junction, respectively. Un-skewed sinusoidal patterns are obtained, with no sign of jumps. Figures S2e and S2f show the line cuts in Figs. S2c and S2d at  $I_b=0$ , respectively. No oscillatory structure can be resolved within the resolution limit, indicating that the gap is never closed at zero bias.

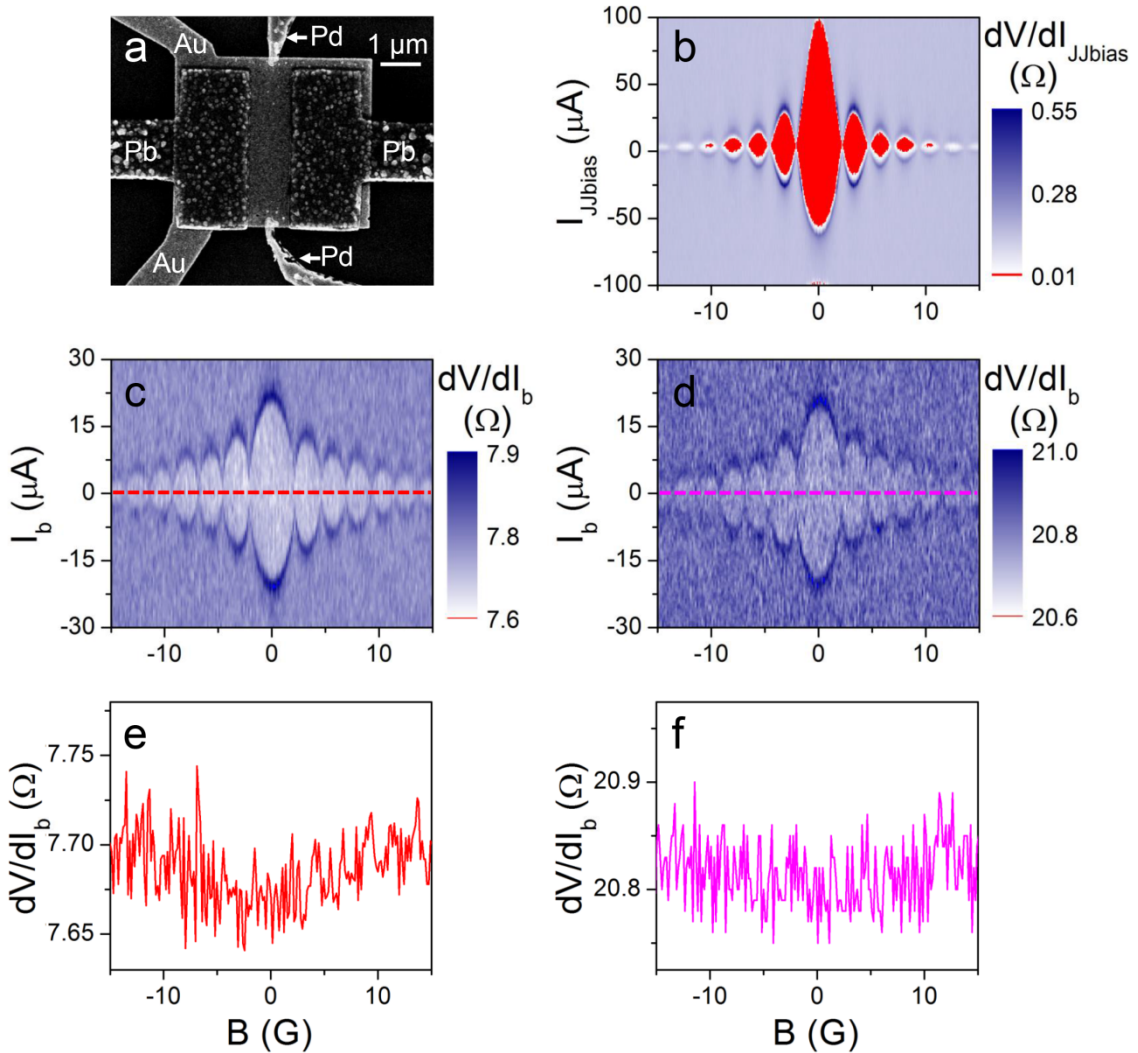

**FIG. S2 |** (a) SEM image of the Pb-Au-Pb device, with two point contact-like Pd electrodes connecting to the two ends of the junction. (b) Fraunhofer diffraction pattern of the Pb-Au-Pb Josephson junction, as functions of magnetic field  $B$  and current  $I_{JJbias}$  flowing through the junction. The red colored area represents the zero-resistance state. (c) and (d) The measured contact resistance by the Pd electrodes at the upper and lower ends of the junction, respectively, as functions of magnetic field and the bias current injected into each contact. (e) and (f) the line cuts (c) and (d) at  $I_b=0$ , respectively. The transport measurements were performed at  $\sim 200$  mK.

The  $dV/dI_b$  of Au-Pd point contacts has a low-resistance state near the zero bias. There the conductance enhancement is caused by Andreev reflection at the S-N interface, and can be explained within the BTK theory (G. E. Blonder, M. Tinkham, M. T. Klapwijk, Phys. Rev. B 25, 4515 (1982)). The envelope of the low-resistance state in Figs. S2c and S2d is related to a characteristic critical current, which is not but the local excess current of the S-N interface:  $I_e \propto (\Delta/eR) \tanh(V/2k_B T)$ , where  $R$  is the normal-state resistance of the point contact, and  $\Delta$  is the local minigap in superconducting Au (see A. Barone, *Physics and application of the Josephson effect*. John Wiley and Sons, Inc. 1982). In the large- $V$  limit, the shape of the envelope is determined by  $\Delta$ .

The shape of the low-resistance state in Figs. S2c and S2d is similar to the Fraunhofer pattern shown in Fig. S2b. However, it has to be pointed out that the measured pattern by each Pd contact only probes the local S-N-like transition with increasing  $I_b$ , not the Fraunhofer pattern which is a globally integrated feature. This conclusion is reasonable because the bias current used in the contact resistance measurements is significantly smaller than the total critical supercurrent of the Pb-Au-Pb junction.

### 3. The mechanism of $\pi$ phase shift in a single Josephson junction

In the following we will show that near the node fields of the Fraunhofer pattern the phase constant of a single Josephson junction can be freely adjusted between 0 and  $\pi$ , both states have the same total energy and carry zero net current. The total energy of the two states is:

$$E_J = \begin{cases} \frac{\Delta_0}{W} \int_{-\frac{W}{2}}^{\frac{W}{2}} [1 - \cos(\frac{2\pi\phi}{\phi_0})] dx & (\text{without } \pi \text{ phase shift}) \\ \frac{\Delta_0}{W} \int_{-\frac{W}{2}}^{\frac{W}{2}} [1 - \cos(\frac{2\pi\phi}{\phi_0} \pm \pi)] dx & (\text{with } \pi \text{ phase shift}) \end{cases}$$

$$= \begin{cases} \Delta_0 [1 - \frac{\sin(\pi\phi/\phi_0)}{\pi\phi/\phi_0}] & (\text{without } \pi \text{ phase shift}) \\ \Delta_0 [1 + \frac{\sin(\pi\phi/\phi_0)}{\pi\phi/\phi_0}] & (\text{with } \pi \text{ phase shift}) \end{cases}$$

where  $\Delta_0$  is a constant,  $\phi=BHx$  is the flux in the junction area,  $H$  is the effective length and  $W$  the width of the junction.

Shown in Fig. S3 is the calculated  $E_J$  of the two states with (red) and without (blue) the  $\pi$  phase shift. In order for the system to trace the lowest energy state, a  $\pi$  phase shift will happen at the node fields of the Fraunhofer pattern, accompanied with the reverse of the screening supercurrent against the Josephson vortex.

It should be noted that the  $\pi$  phase shift in a single Josephson junction as discussed above is different from the  $\pi$  phase shift in a rf-SQUID constructed on the surface of TI (Y. Pang et.al., arXiv:1503.00838v2). In the rf-SQUID structure, there is no adjustable phase different constant, since the two superconducting pads are connected by the superconducting ring. The  $\pi$  phase shift observed there could only be attributed to a topologically nontrivial mechanism – quasiparticle-poisoning-mediated inter-branch switching between two  $4\pi$ -periodic EPRs with opposite parities.

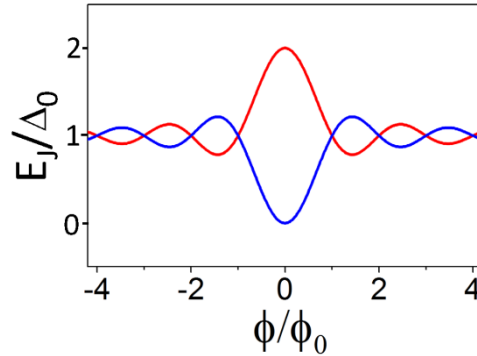

**FIG. S3** | Two branches of energy-flux relation of the Josephson junction.

#### 4. The minigap in S-N-S Josephson junctions with different transparency to quasiparticle process

The minigap is the energy separation between the two lowest-energy branches of Andreev bound states whose EPRs are:

$$E_n = \pm \Delta_0 [1 - D_n \sin^2(\varphi/2)]^{1/2}$$

where  $E_n$  and  $D_n$  are the Josephson energy and the transmission coefficient of the  $n^{\text{th}}$  allowed mode of the quasiparticles in the junction, respectively. The curves plotted in Fig. S4 are the calculated  $E_n$  at several different  $D_n$ . It can be seen that the minigap is significantly not fully closed even if the transmission coefficient is as high as 0.99. Full gap closing only happens when  $D_n=1$ .

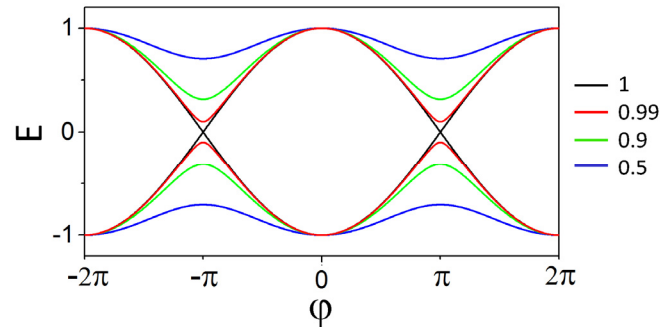

**FIG. S4** | The energy-phase relation of the lowest-energy Andreev bound states at several different transmission coefficient.

## 5. Estimation of the effective junction area after considering flux compression

In Fig. S5 we illustrate how the effective junction area of the device shown in Fig. 1 of the main manuscript is calculated after considering flux compression and stray supercurrent distribution.

As illustrated in the upper left panel of Fig. S5, below  $H_{c1}$  the magnetic field cannot penetrate into the bulk of superconducting Pb film other than within the penetration depth. The flux lines will therefore be pushed away from the Pb electrodes and focused in the junction area, making the effective junction area larger.

On the other hand, we know that superconductivity will be induced on the TI surface by proximity effect, spreading away to a distance of micron (Qu, F. et al., Sci. Rep. 2, 339 (2012); Yang, F. et al., Phys. Rev. B 86, 134504 (2012)). Therefore, the TI surface near Pb electrodes will be able to carry stray supercurrents.

After taking into consideration of the above facts, we employed an empirical method of estimating the effective junction area as shown in the right panel of Fig. S5. By comparing with the effective area drawn from the Fraunhofer pattern measurements, the effective area estimated by this method turns out to be accurate, with an error less than 20%.

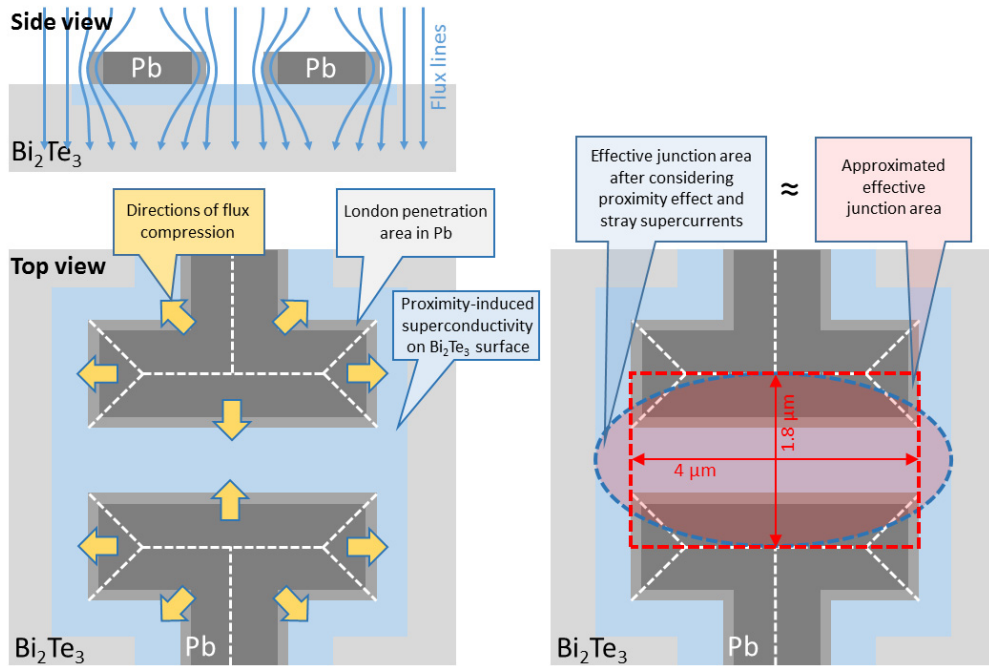

**FIG. S5 | Upper left panel:** Side view for flux compression. **Lower left panel:** Top view for flux compression. The flux in each area defined by white dashed lines will be compressed away along the arrowed directions. **Right panel:** Our empirical method of estimating the effective junction area after considering flux compression and stray supercurrent distribution.
